# Supplementary material for: From Idea to Co-Creation: A Planner-Actor-Critic Framework for Agent Augmented 3D Modeling
Source: arXiv:2601.05016 source file (2026-01-08)
Supplement: Supplementary file 1 [file Experiments_sm.pdf]

# Experiment 1- Construct a low-poly classic car using only primitive shapes

**iteration 1:**

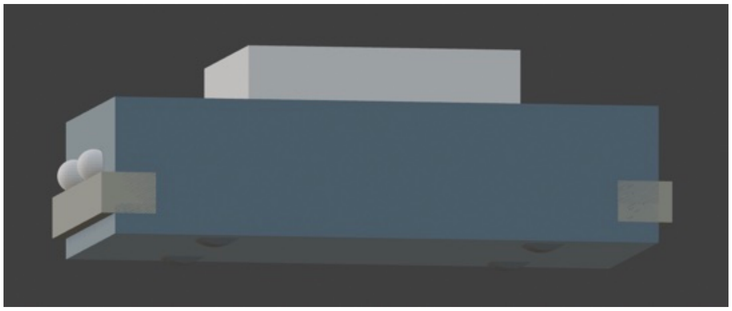

**iteration 2:**

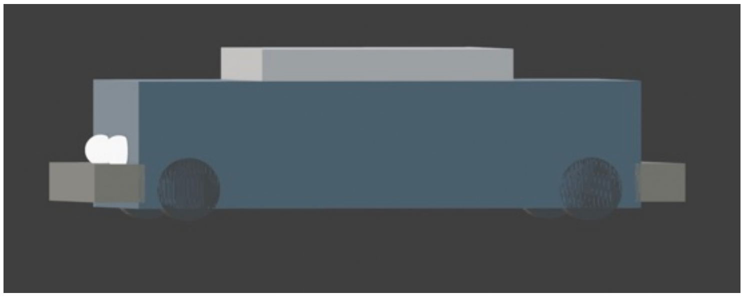

**iteration 3:**

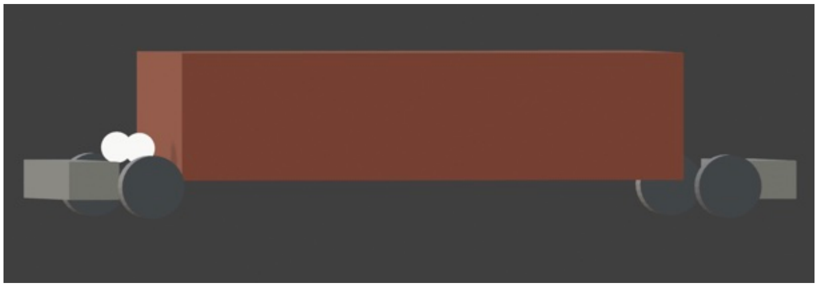

**iteration 4:**

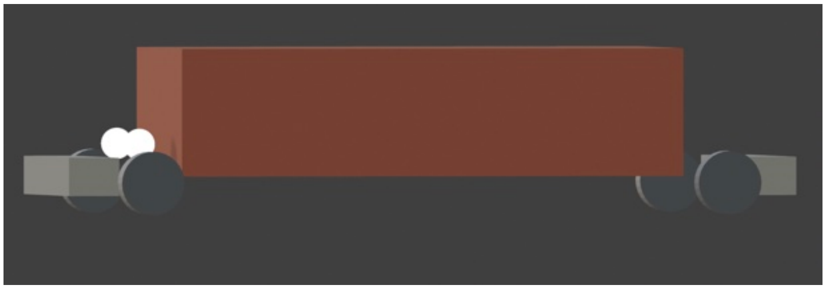

**iteration 5:**

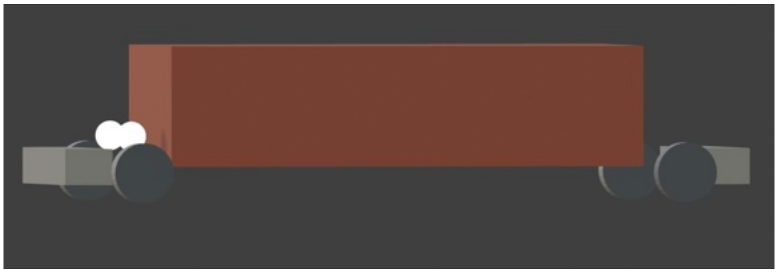

# Experiment 2- Construct a low-poly classic car using only primitive shapes

**Iteration 1:**

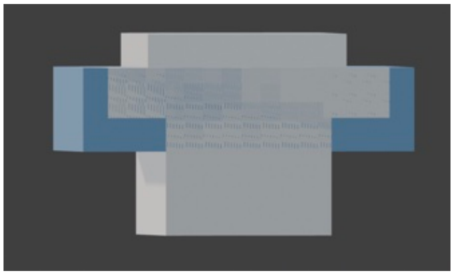

**Iteration 2:**

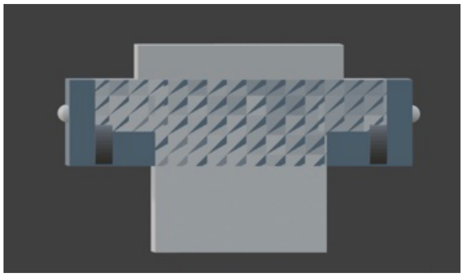

**Iteration3:**

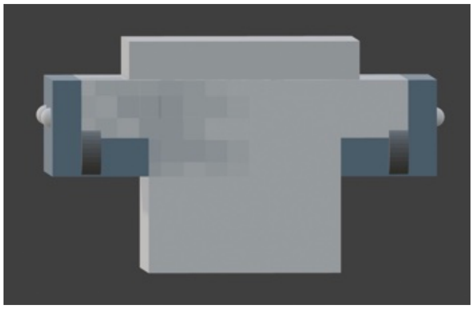

**Iteration4:**

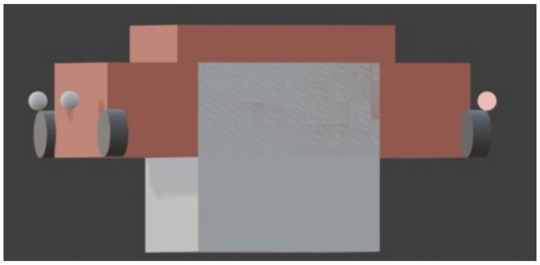

**Iteration5:**

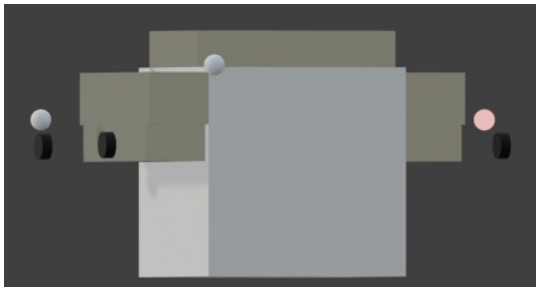

## Experiment 3- Construct a low-poly classic car using only primitive shapes

**iteration 1:**

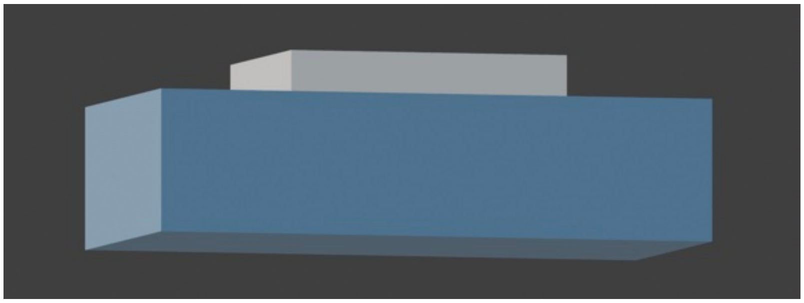

**iteration 2:**

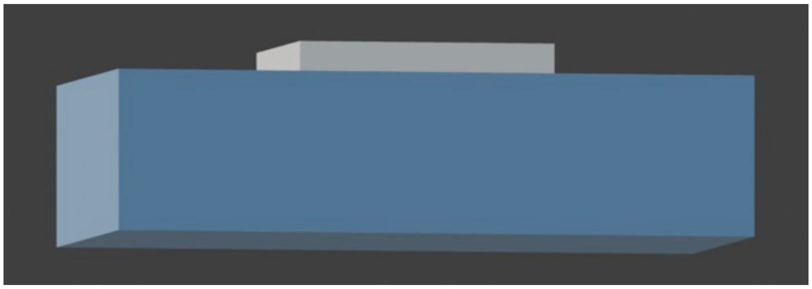

**iteration 3:**

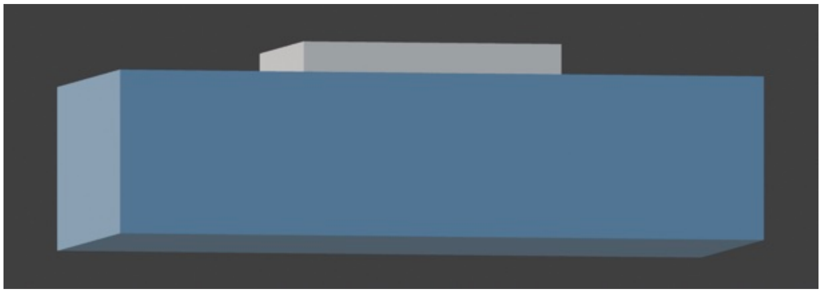

**iteration 4:**

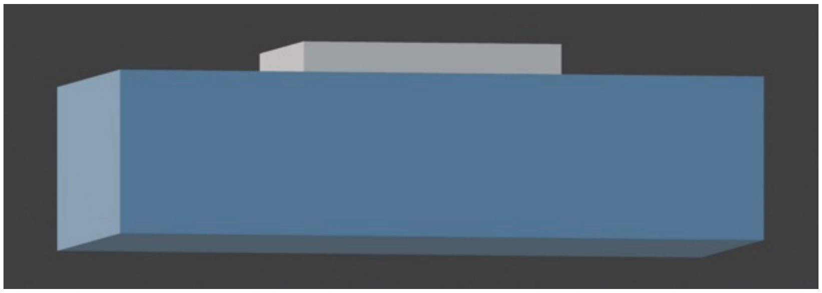

**iteration 5:**

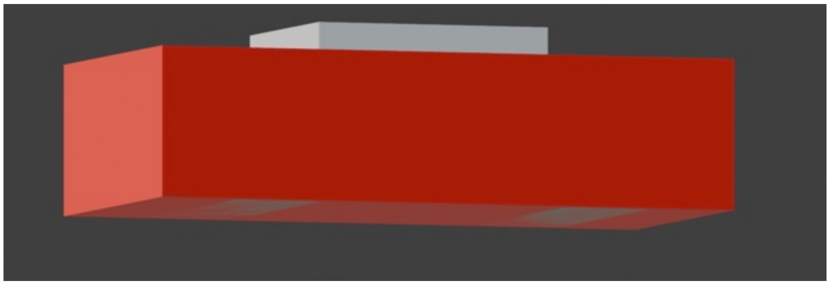

# Experiment 4- Construct a low-poly classic car using only primitive shapes

**iteration 1:**

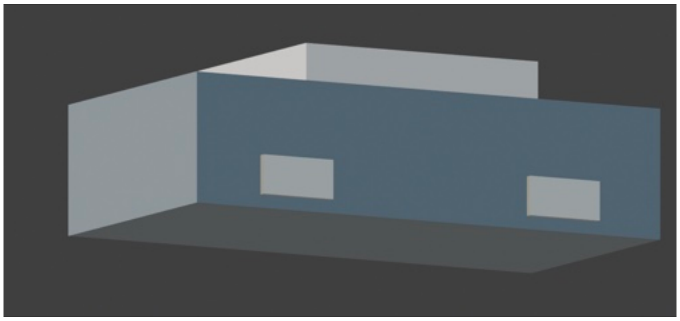

**iteration 2:**

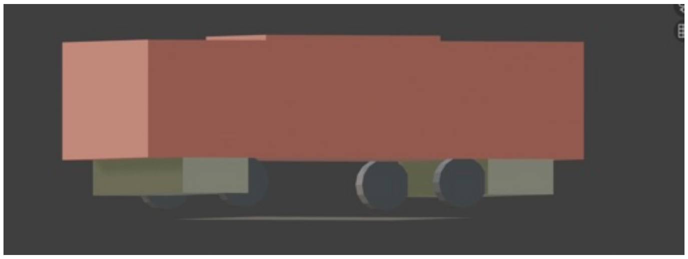

**iteration 3:**

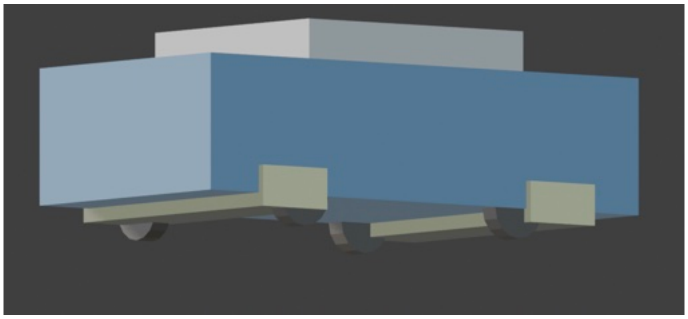

**iteration 4:**

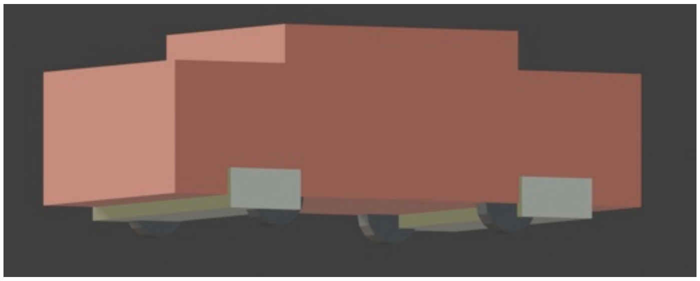

**iteration 5:**

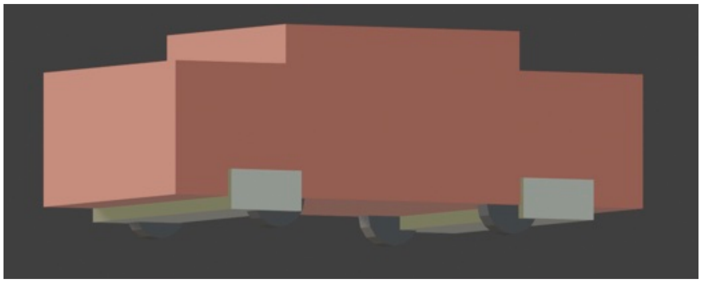

# Experiment 5- Construct a low-poly classic car using only primitive shapes

Iteration 1

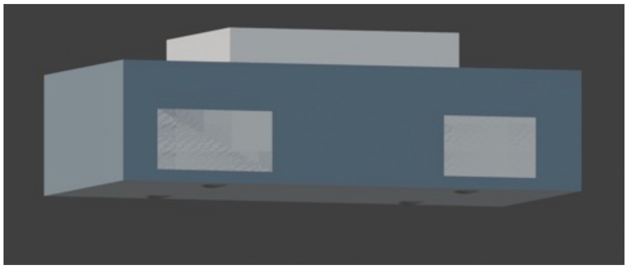

iteration 2:

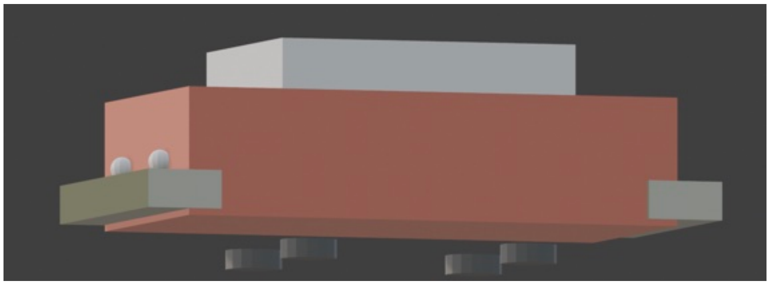

iteration 3:

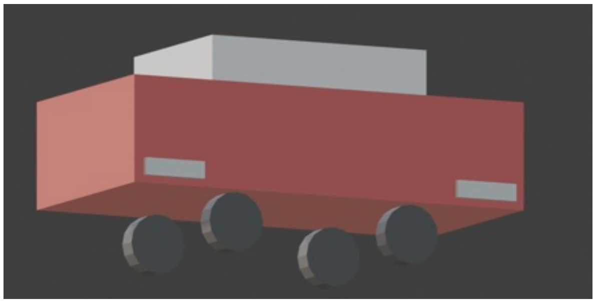

iteration 4:

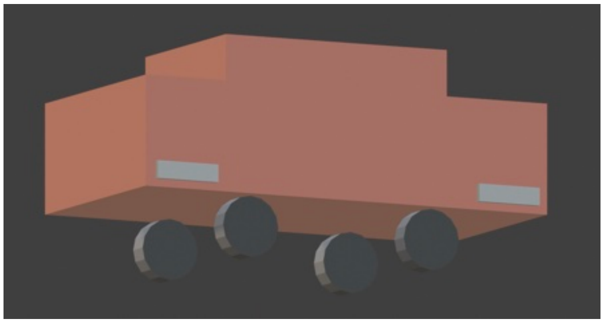

iteration 5:

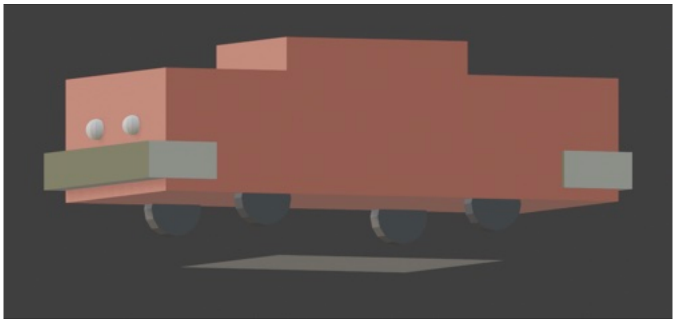

# Experiment 1:Model a low-poly birthday cake with visible layers and candles

| | |
|---|---|
| **Iteration 1:** 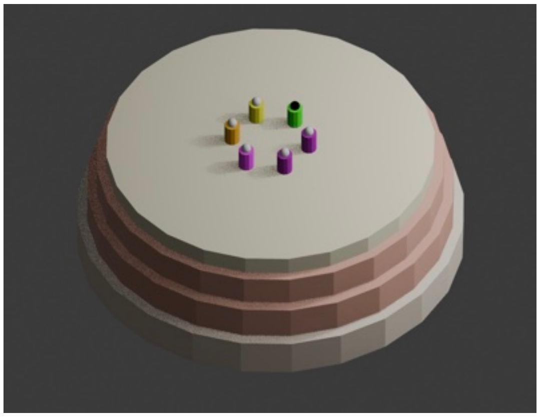 | **Iteration 2:** 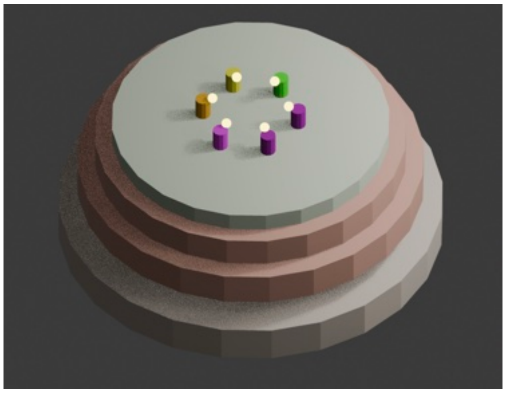 |
| **Iteration 3:** 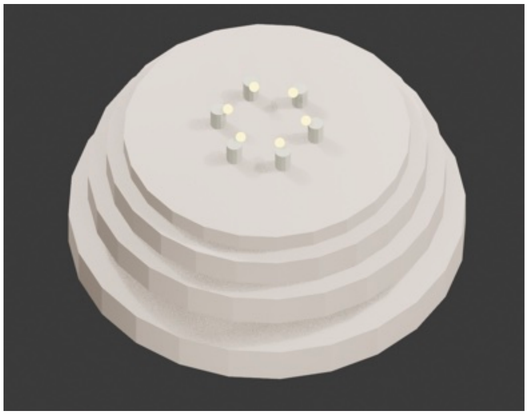 | **Iteration 4:** 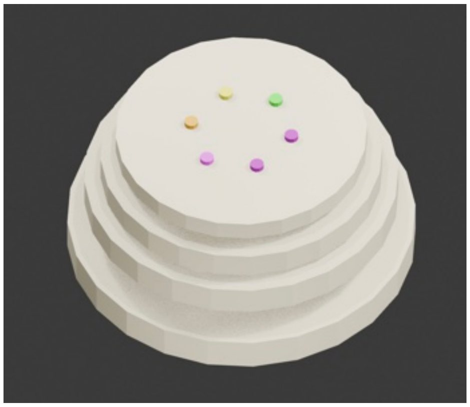 |
| **Iteration 5:** 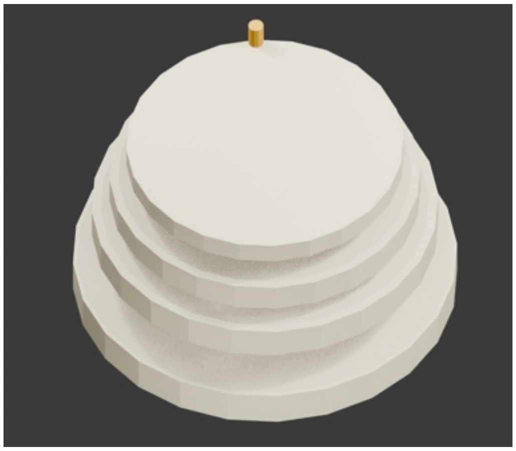 | |

# Experiment 2:Model a low-poly birthday cake with visible layers and candles

| | |
|---|---|
| **Iteration 1:**<br>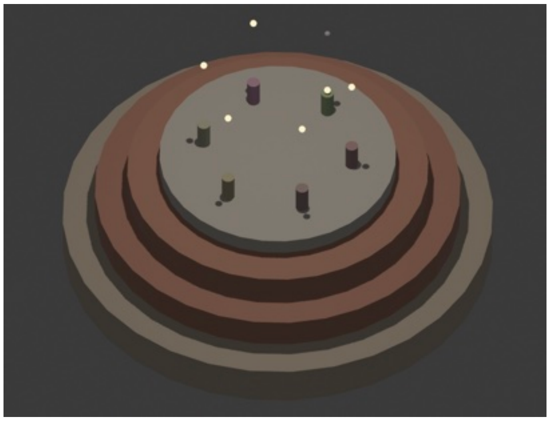 | **Iteration 2:**<br>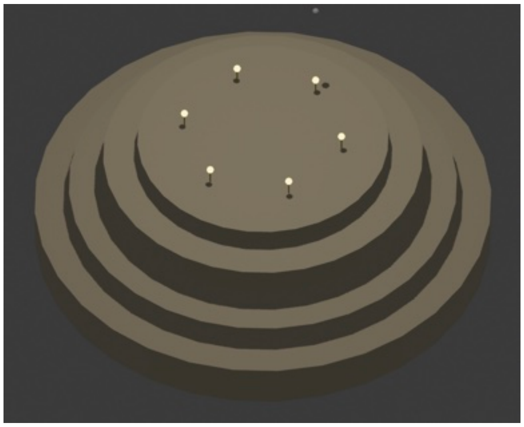 |
| **Iteration 3:**<br>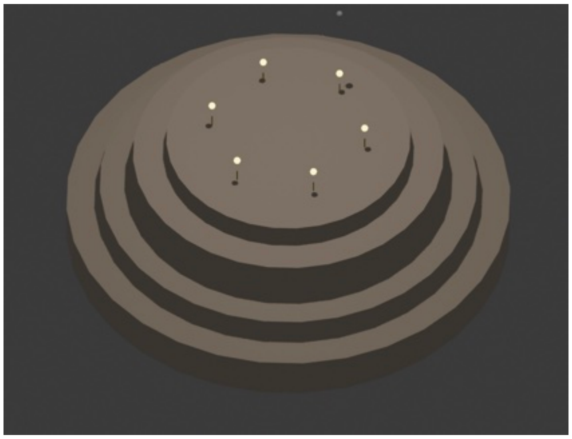 | **Iteration 4:**<br>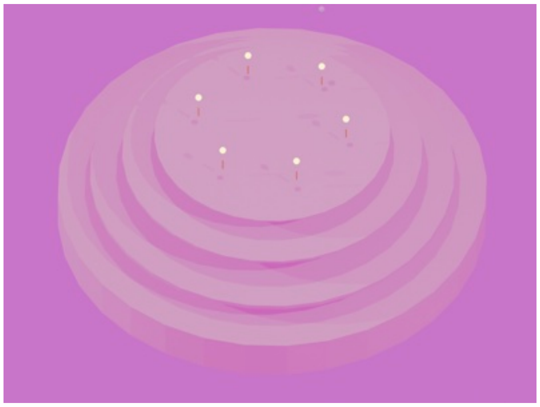 |
| **Iteration 5:**<br>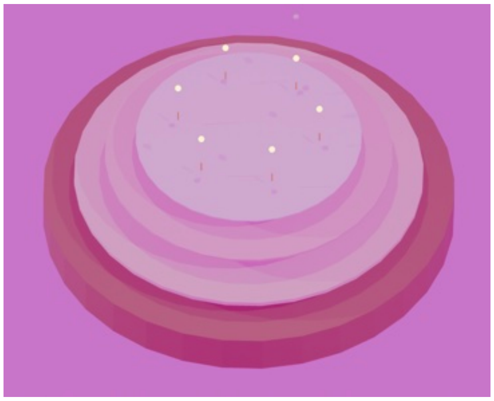 | |

# Experiment 3:Model a low-poly birthday cake with visible layers and candles

| | |
|---|---|
| **Iteration 1:**<br>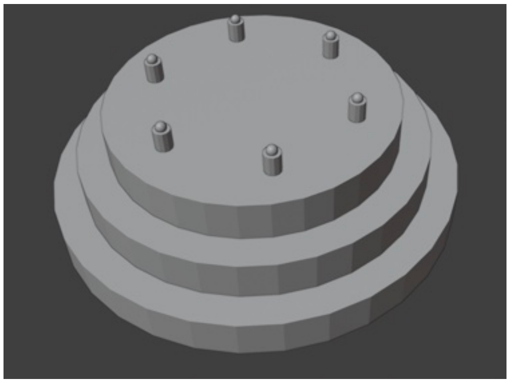 | **Iteration 2:**<br>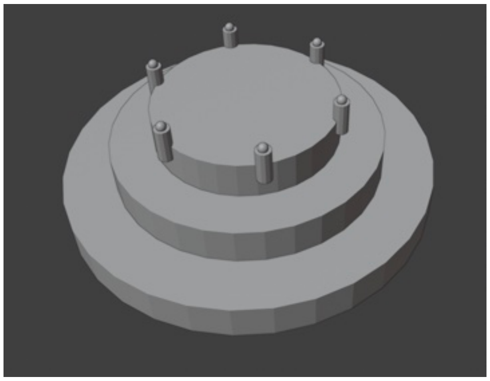 |
| **Iteration 3:**<br>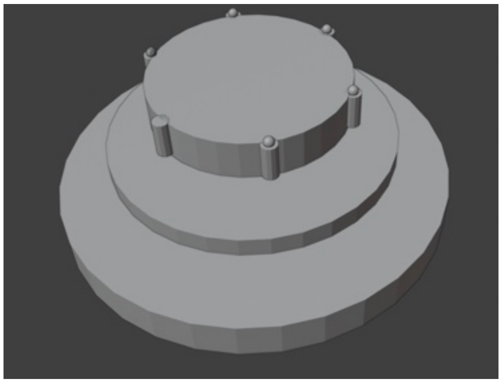 | **Iteration 4:**<br>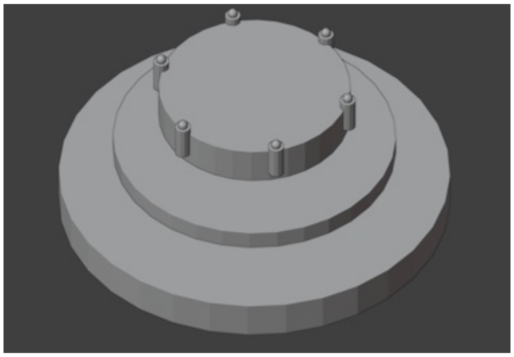 |
| **Iteration 5:**<br>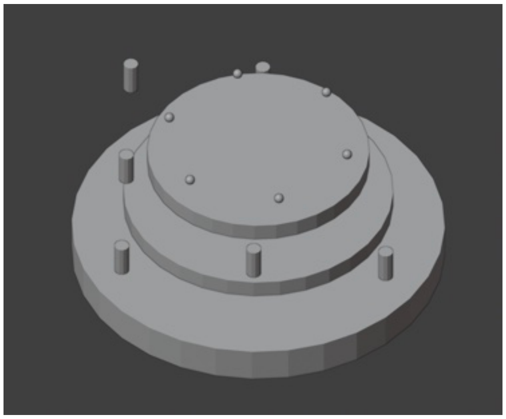 | |

# Experiment 4:Model a low-poly birthday cake with visible layers and candles

| | |
|---|---|
| **Iteration 1:** 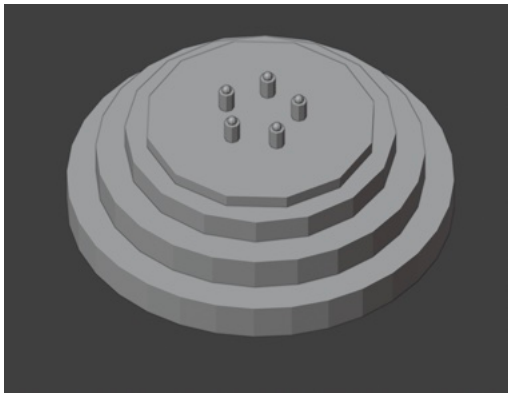 | **Iteration 2:** 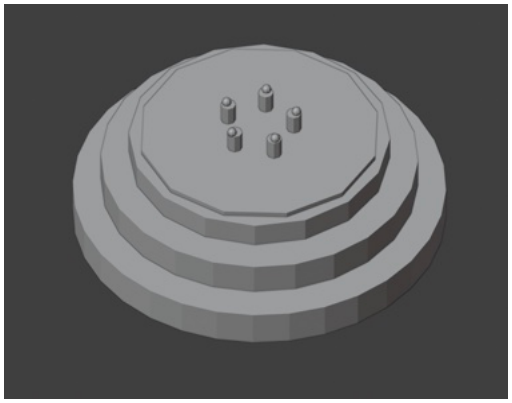 |
| **Iteration 3:** 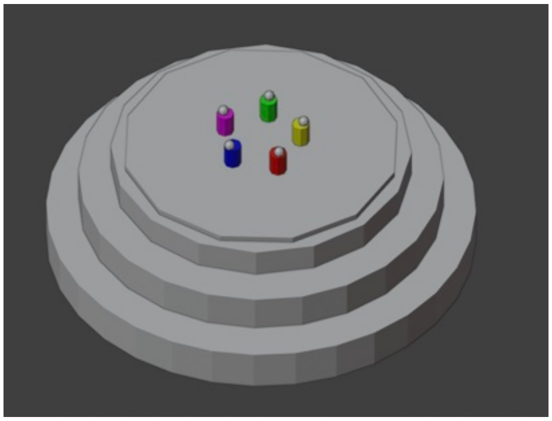 | **Iteration 4:** 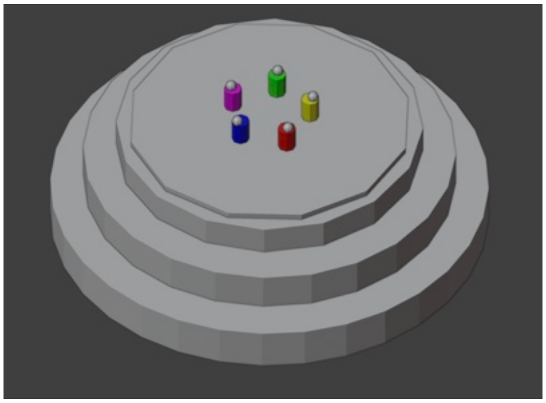 |
| **Iteration 5:** 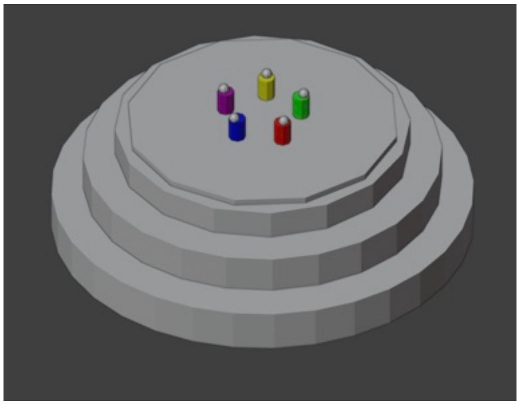 | |

# Experiment 5:Model a low-poly birthday cake with visible layers and candles

| | |
|---|---|
| **Iteration 1:**<br>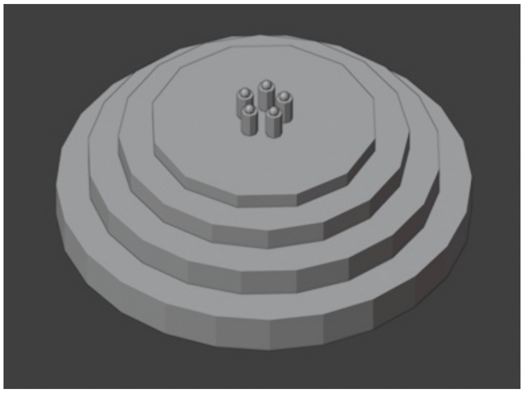 | **Iteration 2:**<br>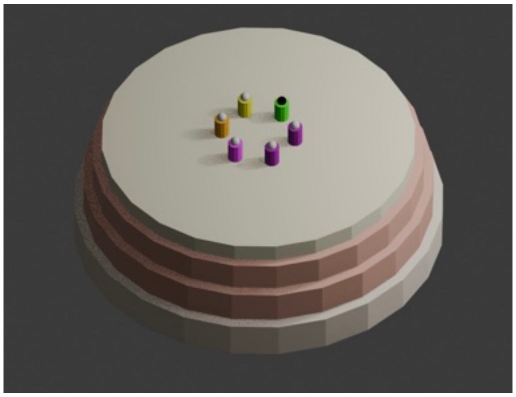 |
| **Iteration 3:**<br>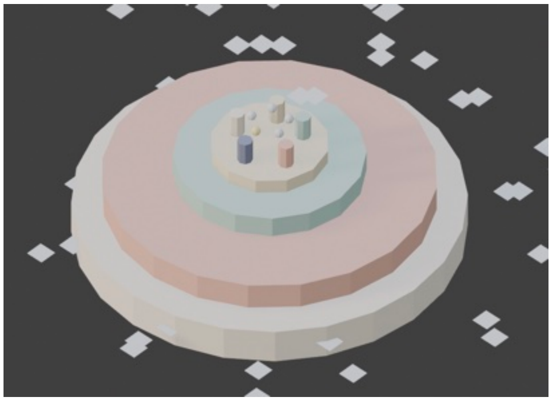 | **Iteration 4:**<br>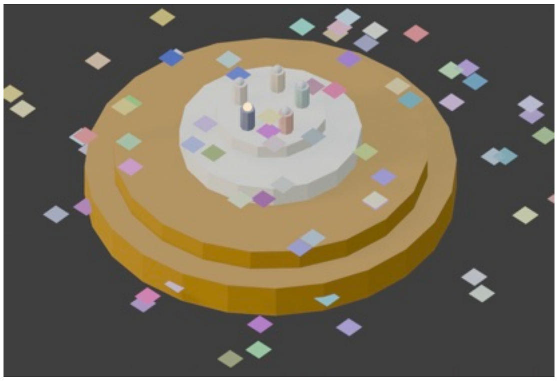 |
| **Iteration 5:**<br>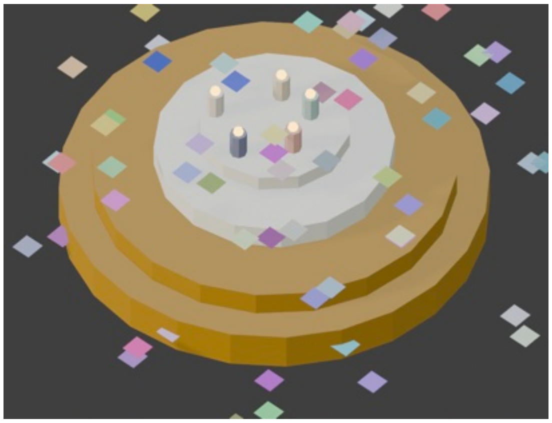 | |

# Experiment 1: Create a low-poly square dining table with four legs

| | |
|---|---|
| **Iteration 1:**<br>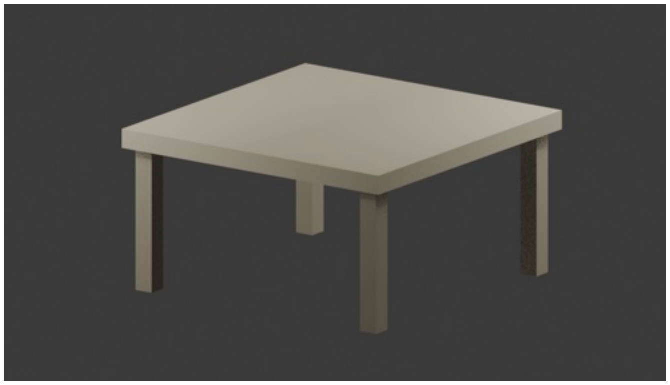 | **Iteration 2:**<br>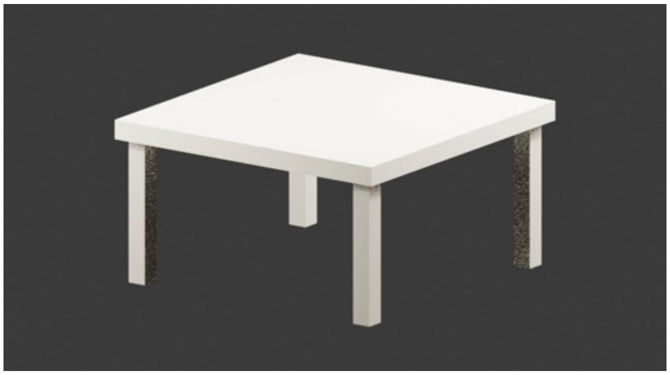 |
| **Iteration 3:**<br>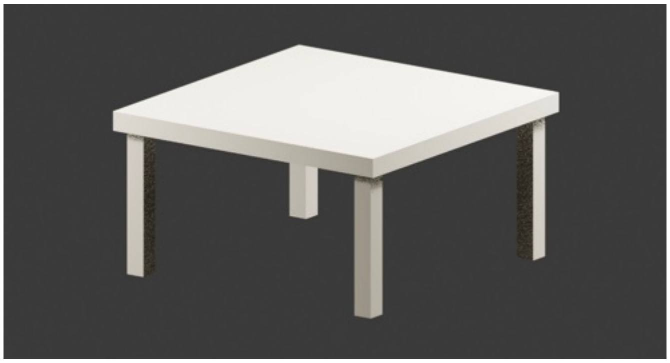 | **Iteration 4:**<br>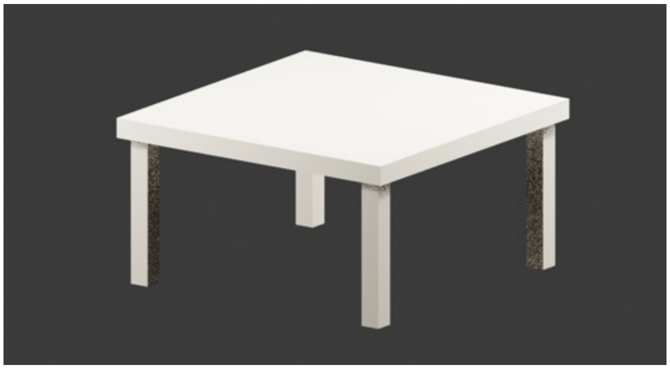 |
| **Iteration 5:**<br>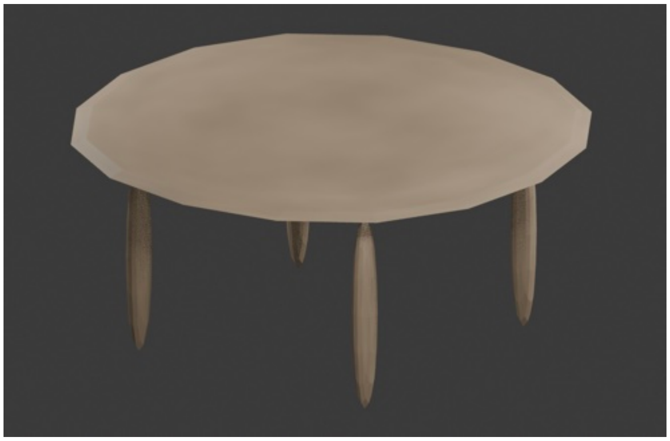 | |

## Experiment 2: Create a low-poly square dining table with four legs

| | |
|---|---|
| **Iteration 1:** 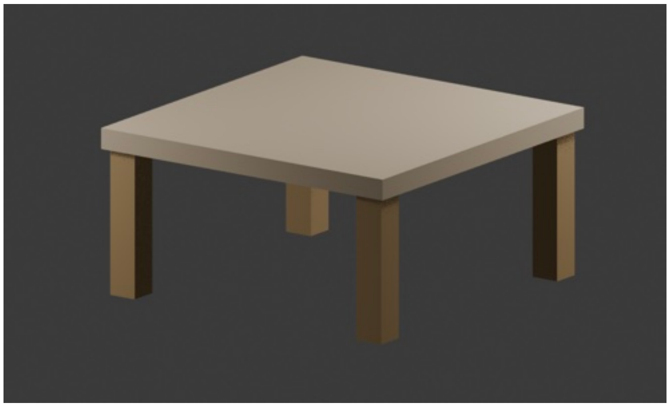 | **Iteration 2:** 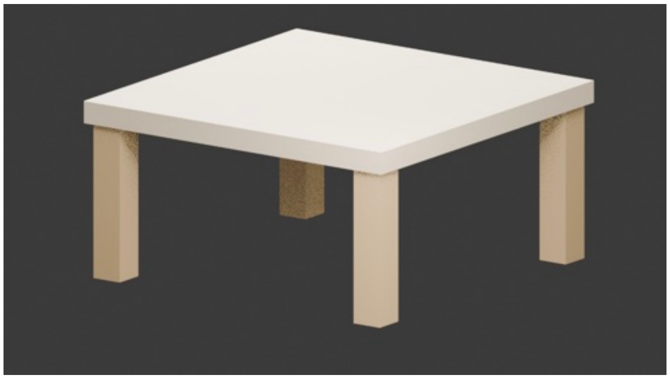 |
| **Iteration 3:** 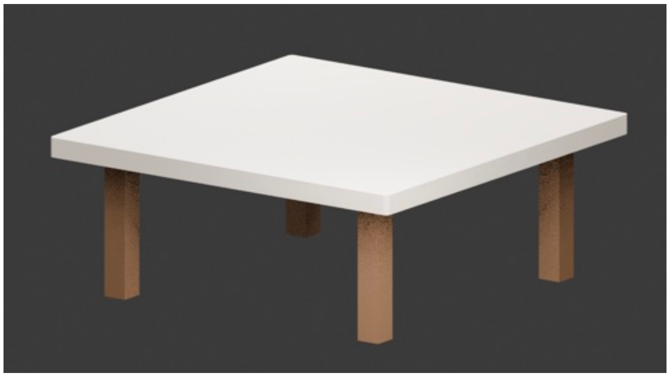 | **Iteration 4:** 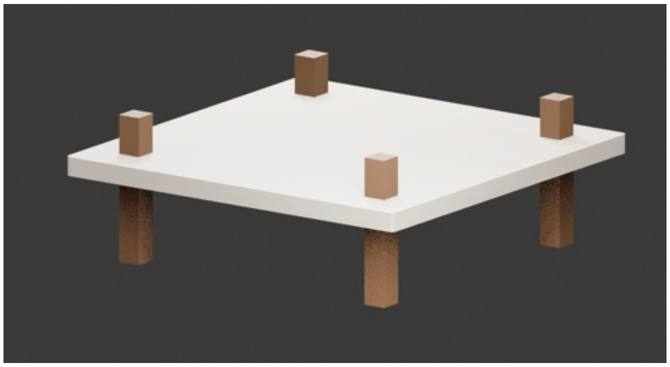 |
| **Iteration 5:** 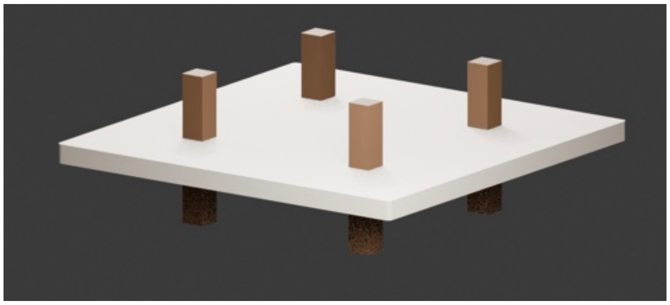 | |

# Experiment 3: Create a low-poly square dining table with four legs

| | |
|---|---|
| **Iteration 1:**<br>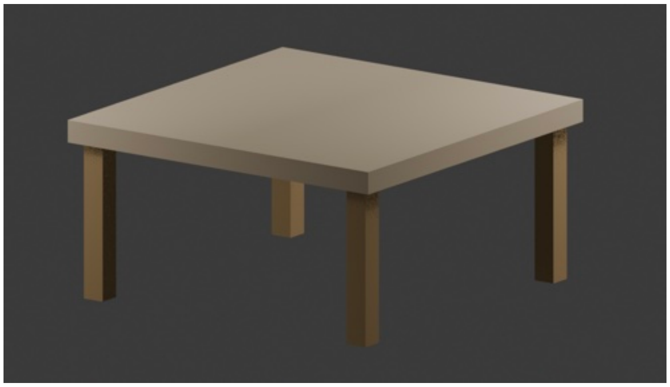 | **Iteration 2:**<br>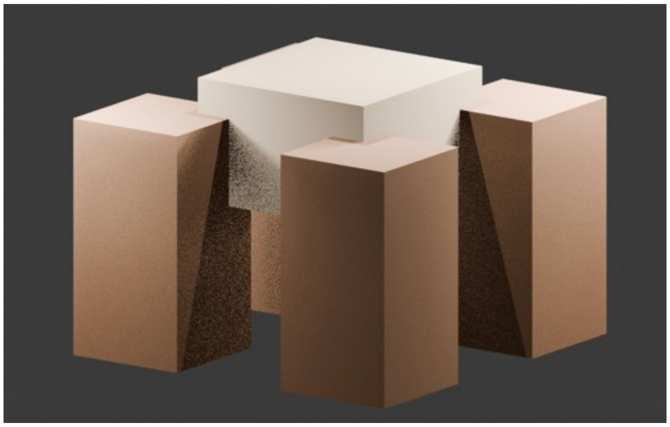 |
| **Iteration 3:**<br>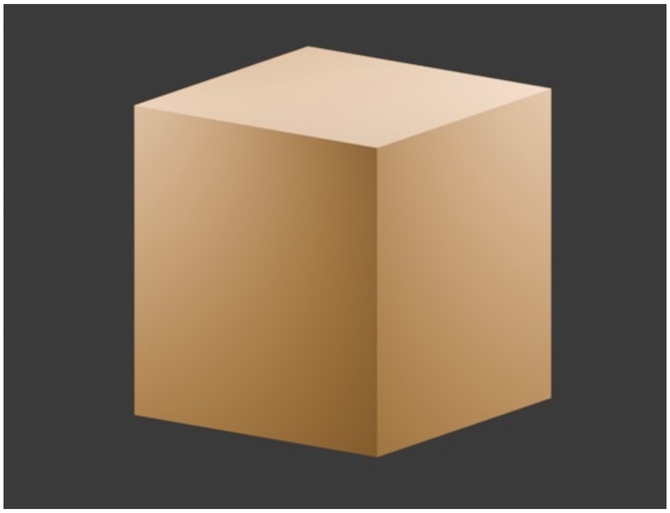 | **Iteration 4:**<br>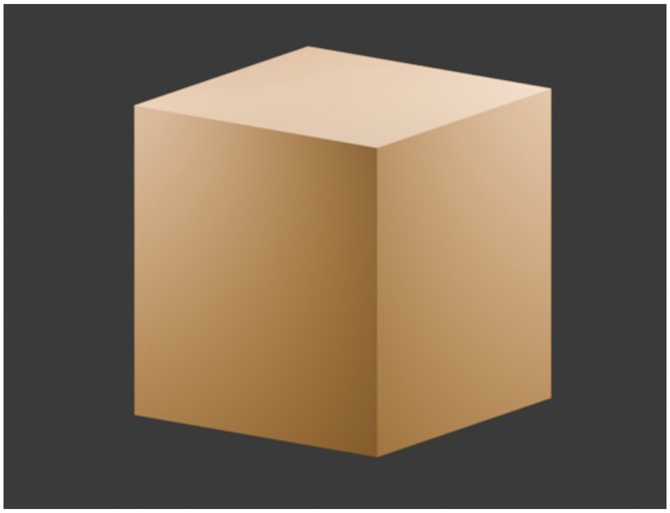 |
| **Iteration 5:**<br>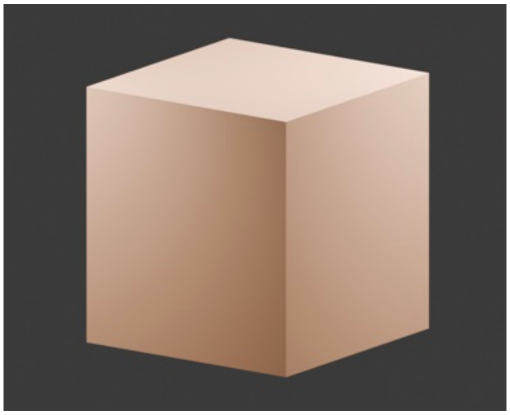 | |

# Experiment 4: Create a low-poly square dining table with four legs

| | |
|---|---|
| **Iteration 1:** 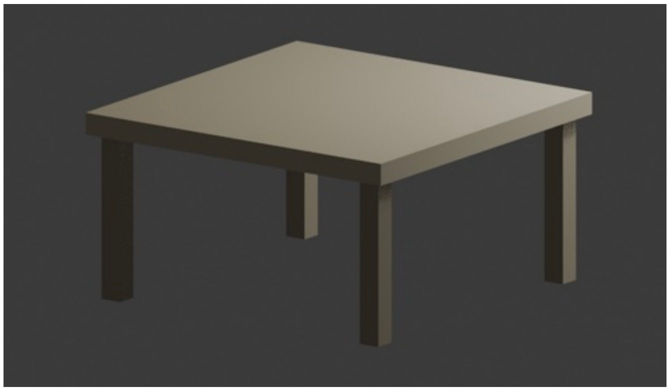 | **Iteration 2:** 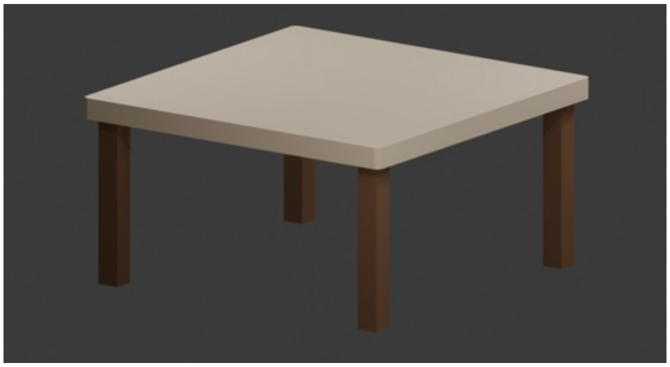 |
| **Iteration 3:** 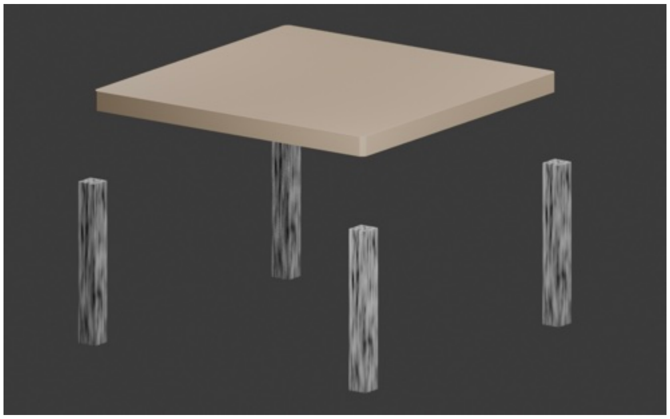 | **Iteration 4:** 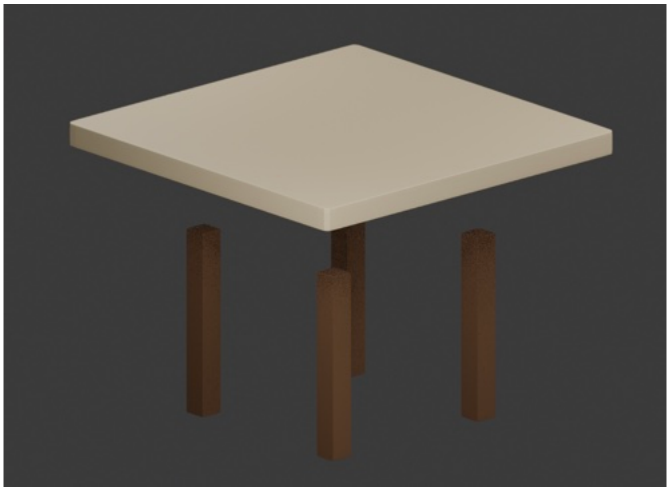 |
| **Iteration 5:** 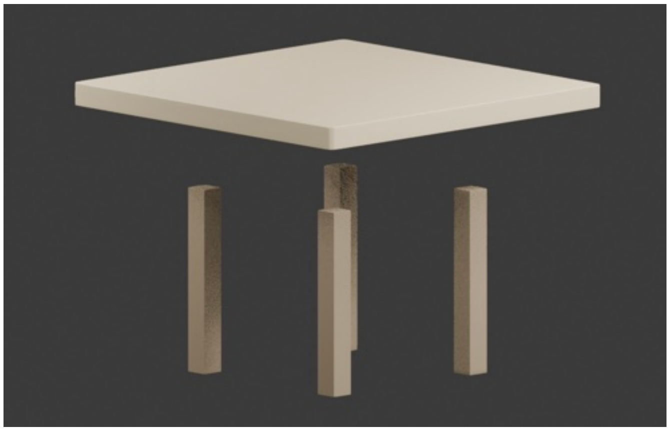 | |

## Experiment 5: Create a low-poly square dining table with four legs

| | |
|---|---|
| **Iteration 1:** 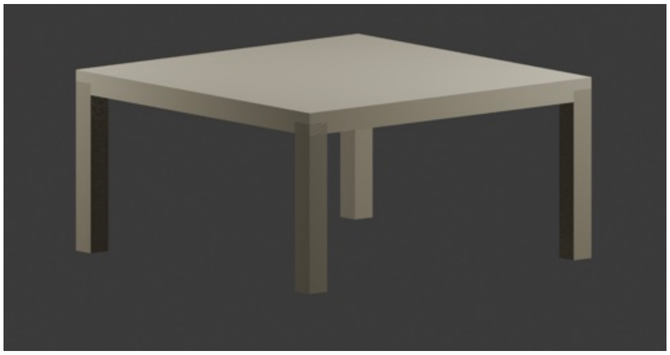 | **Iteration 2:** 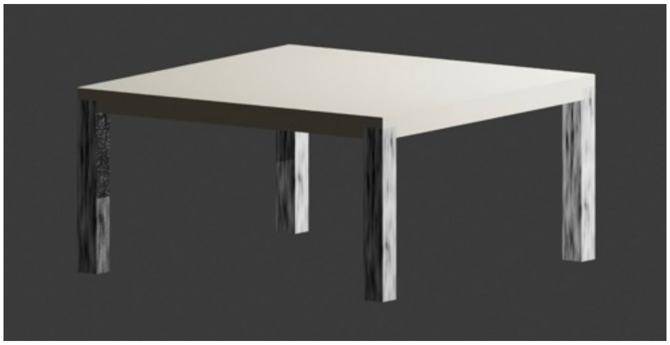 |
| **Iteration 3:** 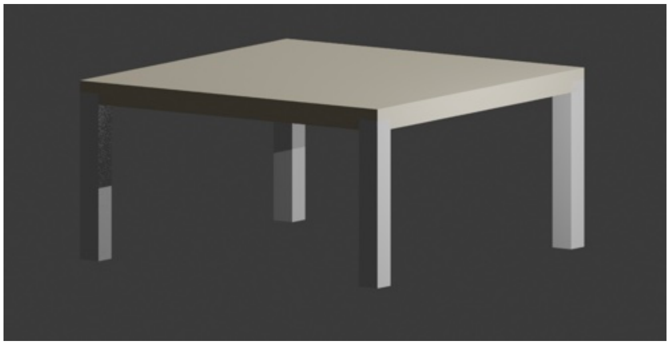 | **Iteration 4:** 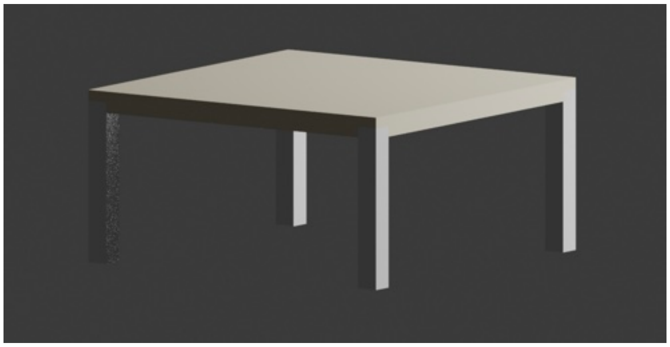 |
| **Iteration 5:** 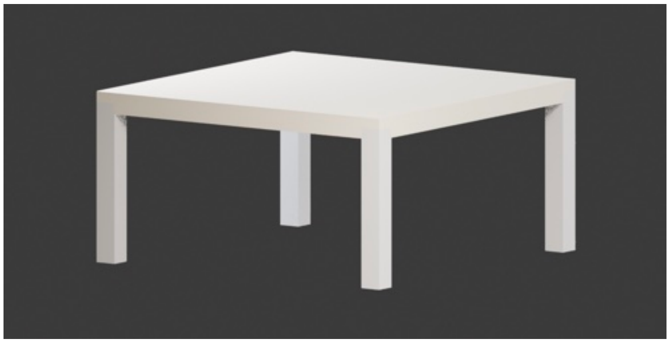 | |
